# Supplementary material for: Online Uniform Sampling: Randomized Learning-Augmented Approximation Algorithms with Application to Digital Health
Source: arXiv:2402.01995 source file (2024-10-19)
Supplement: Supplementary file 1 [file appendix6.tex]

\label{lower}
We define an auxiliary problem based on the \textit{button problem} in \citet{shin2023improved}, which we call the \textit{new button problem}. 

Suppose we have an ordered list of $m $ buttons where some buttons are designated as \textit{targets}. There exists a button $J \leq m$ such that buttons $1$ to $(J-1)$ are not targets, but buttons $J$ to $m$ are all targets.

However, the first target button $J$ is unknown. To learn whether a button $j\in [m]$ is a target, we must click it. Every time we click a button, we collect a reward $r_j$. The rewards of the buttons are given at the beginning. The rewards are monotone increasing.
% Let $b^{(1)} = b$. In the first round, the rewards are $r_1^{(1)} = \frac{b^{(1)}}{b}, r_2^{(1)} = \frac{b^{(1)}}{b+1}, \ldots, r_m^{(1)} = \frac{b^{(1)}}{T}$. The price of button $J$ is $r_J^{(1)}=\frac{b^{(1)}}{J}$. 
% For the next round, the rewards become $r_1^{(2)} = \frac{b^{(2)}}{b-1}, r_2^{(2)} = \frac{b^{(2)}}{b}, \ldots, r_m^{(2)} = \frac{b^{(2)}}{T-1}$, where $b^{(2)} = b^{(1)} - r_{j^{(1)}}^{(1)}$ where $j^{(1)} \in [m]$ represents the button selected in the first round. In addition, in the second round, we need to pay a price $c^{(2)} = \frac{1}{\tau^*} \ln \frac{r_{j^{(1)}}^{(1)}}{r_{j^{(2)}}^{(2)}}$ for switching to a different button.  The process is repeated for the rest of the rounds until it reaches $\tau^*$ rounds. 
The objective is to maximize the total rewards. 

We want to show that a lower bound for the button problem immediately extends to give (almost) the same lower bound for the online uniform risk times sampling problem, which can stated as the following lemma.

\begin{lemma}
  Suppose there exists a randomized $\rho$-competitive algorithm for the online uniform risk times sampling algorithm. Then, for all constant $\epsilon \in (0,1)$, there exists a randomized $(\rho+\epsilon)$-competitive algorithm for the new button problem. 
\end{lemma}

We first present the reduction algorithm from Algorithm 1 to the new button problem. Let $\mathcal{A}$ denote our non-learning augmented randomized algorithm (Algorithm 1) for the online uniform risk times sampling problem. The reduction algorithm runs $\mathcal{A}$ on the new button problem. 

Note that, the algorithm $\mathcal{A}$ runs in stages.
At each stage $k$, $\mathcal{A}$ generates $(p^{(k)}, \tilde{\tau}^{(k)})$, we further calculate a budget utilization variable $U^{(k)} = p^{(k)} \cdot \tilde{\tau}^{(k)} - \frac{1}{\tau^*}\ln \frac{p^{(k-1)}}{p^{(k)}}$. Problem: $\tau^*$ is unknown, can we use $T$ instead?
We click the \textit{first} button whose reward exceeds $U^{(k)}$. If the clicked button is a target button, we terminate $\mathcal{A}$. 

In order to ensure that the algorithm always terminates, we require that once the total rewards incurred by $\mathcal{A}$ becomes at least $b$, we click the last button and terminate. 
Let $\operatorname{SOL}$ be the total benefit incurred by the reduction algorithm. We have that $\operatorname{SOL}$ is no smaller than the total benefit incurred by $\mathcal{A}$. 

Then, it suffices to show that the next lemma holds.

\begin{lemma}
    This reduction algorithm is a randomized $(\chi(T)  - \epsilon)$-competitive algorithm for the new button problem. 
\end{lemma}

\begin{proof}
Let $c(\mathcal{A})$ denote the objective value incurred by $\mathcal{A}$ for the online uniform risk times sampling problem. By design of the reduction algorithm, we always click the first button whose reward exceeds $U^{(k)}$. 
% \xueqing{How to argue the price of switching buttons is close to the penalty term? e.g., $\frac{1}{\tau^*} \log \frac{r_{j^{(1)}}^{(1)}}{r_{j^{(2)}}^{(2)}}$ and $\frac{1}{\tau^*}\log \frac{p_1}{p_2}$ }
Therefore, we have $\operatorname{SOL} \geq c(\mathcal{A}) \geq b$.
\end{proof}

% \xueqing{1) do we need the additional $\epsilon$? 2) is forced termination necessary? }

% A tentative theorem we have trying to prove: 
\begin{theorem}
    For all constant $\epsilon > 0$, no randomized algorithm can achieve a competitive ratio of $e - \epsilon$.
\end{theorem}

We formulate the following LP whose value constitutes a lower bound for any randomized algorithm for the new button problem.

\begin{align*}
    \max &~\ \gamma\\
    \operatorname{s.t.} ~\ &\sum_{j=1}^m x_j = 1,\\
         &\sum_{j=t}^m y_{t,j} = x_t + \sum_{j=1}^t y_{j,t}  \quad \forall t = 1,\cdots, m ,\\
         &\\
         &x_j\geq 0, \quad \forall j = 1,\cdots, m,\\
         &y_{t,j} \geq 0 \quad \forall t = 1,\cdots,m, ~\, \forall j = t,\cdots,m.
\end{align*}

The dual of this LP is :

\begin{align*}
    \min &~\ w \\
    \operatorname{s.t.} &
\end{align*}
