# Supplementary material for: Online Uniform Sampling: Randomized Learning-Augmented Approximation Algorithms with Application to Digital Health
Source: arXiv:2402.01995 source file (2024-10-19)
Supplement: Supplementary file 2 [file appendix8.tex]

\label{app_lower}
A standard technique for deriving lower bounds is through Yao's Lemma, which involves demonstrating that there exists a distribution on instances/inputs such that every deterministic algorithm performs poorly.

However, applying this technique to derive lower bounds for OUA is challenging. Firstly, the proof requires calculating the expected objective value for every possible deterministic algorithm. This is complex because each algorithm must satisfy the budget constraint while maximizing the objective. A general form for a deterministic algorithm in OUA involves a sequence of randomization probabilities ($p_1$ to $p_{\tau^*}$), but calculating the expected value without specifying the structure of this sequence is difficult. Furthermore, the non-smooth nature of the objective function and the problem's coverage of three different regimes with either finite or infinite time horizons add to the complexity.

Deriving a lower bound for OUA requires a careful reduction to an auxiliary problem that is easier to handle, as motivated by \citet{shin2023improved}. Since this is the first work addressing the OUA problem and given the limited space, we defer the derivation of the lower bound to future work.
